# Supplementary material for: Product of Orthogonal Spheres Parameterization for Disentangled Representation Learning
Source: arXiv:1907.09554 source file (2019-07-22)
Supplement: Supplementary file 1 [file Supp.tex]

% \documentclass{bmvc2k}
% \usepackage{amsmath}
% \usepackage{graphicx}

% %% Enter your paper number here for the review copy
% \bmvcreviewcopy{1056}

% \title{Supplementary Material}

% % Enter the paper's authors in order
% % \addauthor{Name}{email/homepage}{INSTITUTION_CODE}
% \addauthor{Ankita Shukla}{}{1}
% \addauthor{Sarthak Bhagat}{}{1}
% \addauthor{Shagun Uppal}{}{1}
% \addauthor{Saket Anand}{}{1}
% \addauthor{Pavan Turaga}{}{}
% % Enter the institutions
% % \addinstitution{Name\\Address}
% \addinstitution{
% IIIT- Delhi\\
% Delhi, Inda
% }
% \addinstitution{
%  Arizona State University.\\
%  Arizona, USA
% }

% \runninghead{Student, Prof, Collaborator}{BMVC Author Guidelines}

% % Any macro definitions you would like to include
% % These are not defined in the style file, because they don't begin
% % with \bmva, so they might conflict with the user's own macros.
% % The \bmvaOneDot macro adds a full stop unless there is one in the
% % text already.
% % \def\eg{\emph{e.g}\bmvaOneDot}
% % \def\Eg{\emph{E.g}\bmvaOneDot}
% \def\etal{\emph{et al}\bmvaOneDot}

% \newcommand{\hd}{\rotatebox{90}}
% \newcommand{\todo}[1]{{\color{red}#1}}

% \newcommand{\bbR}{\mathbb{R}}
% \newcommand{\calC}{\mathcal{C}}
% \newcommand{\calX}{\mathcal{X}}
% \newcommand{\calL}{\mathcal{L}}
% \newcommand{\calT}{\mathcal{T}}
% \newcommand{\bx}{\mbox{$\mathbf{x}$}}
% \newcommand{\bz}{\mbox{$\mathbf{z}$}}
% \newcommand{\bA}{\mbox{$\mathbf{A}$}}
% \newcommand{\bJ}{\mbox{$\mathbf{J}$}}
% \newcommand{\bI}{\mbox{$\mathbf{I}$}}
% \newcommand{\bZ}{\mbox{$\mathbf{Z}$}}


% %-------------------------------------------------------------------------
% % Document starts here
% \begin{document}

% \maketitle
% \section{Additional Results}
% \subsection{Effect of Cayley Update}
% As mentioned in the optimization strategy in the paper, the hard constraint imposes the representation to lie on the Stiefel manifold, that is achieved by restoring to a Cayley update step. We empirically validated that adding this constraint along with the soft constraint only boost the convergence of algorithm by reducing the objective in fewer epochs but achieves similar results without this transformation step. This shows that meaningful representations are learned with a simple orthonormality constraint on the latent space block. The results are given in Table \ref{table:map} for 2D Sprites dataset.
% \\
% \input{Sections/map_new.tex}
% \subsection{Interpolation Results}
% Our approach reduces leakage of information regarding one factor of variation into different partitions. Figure \ref{fig:beta_VAE} and \ref{fig:factor_VAE} depict interpolation results where each row is linear interpolation between image in the first column to the last in one of the dimensions of the latent space representation. The fact that we are able to restrict the overlap of attribute information between the 3 partitions when using \textbf{PrOSe} reflects that it is successful in ensuring independence among code vectors along with better reconstructions. 

% \input{Sections/interpolation_beta_factor.tex}

% \begin{figure}[h]
% \begin{center}
% %\includegraphics[width=13cm, height=6cm]{images/Beta_VAE/sprites.png}
% \includegraphics[width=12.5cm, height=6cm]{images/Factor_VAE/celebA.png}
% \end{center}
%   \caption{Interpolation across each of the dimensions of latent space: For CelebA $\beta$-VAE (left) and \textbf{PrOSe}  + $\beta$-VAE (right).}
% \label{fig:factor_VAE}
% \end{figure}
% \\


% % \begin{figure}[h]
% % \begin{center}
% % %\includegraphics[width=13cm, height=6cm]{images/Beta_VAE/sprites.png}
% % \includegraphics[width=6cm,height=4cm]{images/loss_plot/both.png}
% % \end{center}
% %   \caption{Loss plot for total loss with (in grey) and without (in orange) Cayley transform step.}
% % \label{fig:factor_VAE}
% % \end{figure}


% % \subsection{Visualization of Identity Code Vectors}
% % \input{Sections/tsne_mnist_id.tex}

% % \subsection{Clustering Performance}
% % \input{Sections/clustering.tex}



% \end{document}
